# Supplementary material for: [Technical Report] Combining Sampling and Synopses with Worst-Case Optimal Runtime and Quality Guarantees for Graph Pattern Cardinality Estimation
Source: arXiv:2103.13681 source file (2021-03-26)
Supplement: Supplementary file 1 [file appendix.tex]

\vspace*{-0.2cm}
\section*{Appendix}
\vspace*{-0.15cm}
\appendix
